# Supplementary material for: Manipulating and Mitigating Generative Model Biases without Retraining
Source: arXiv:2404.02530 source file (2024-09-17)
Supplement: Supplementary file 1 [file X_supplementary_material.tex]

\section{Additional Precise Prompt Engineering Results}
\begin{figure}
    \centering
    \includegraphics[width=\linewidth]{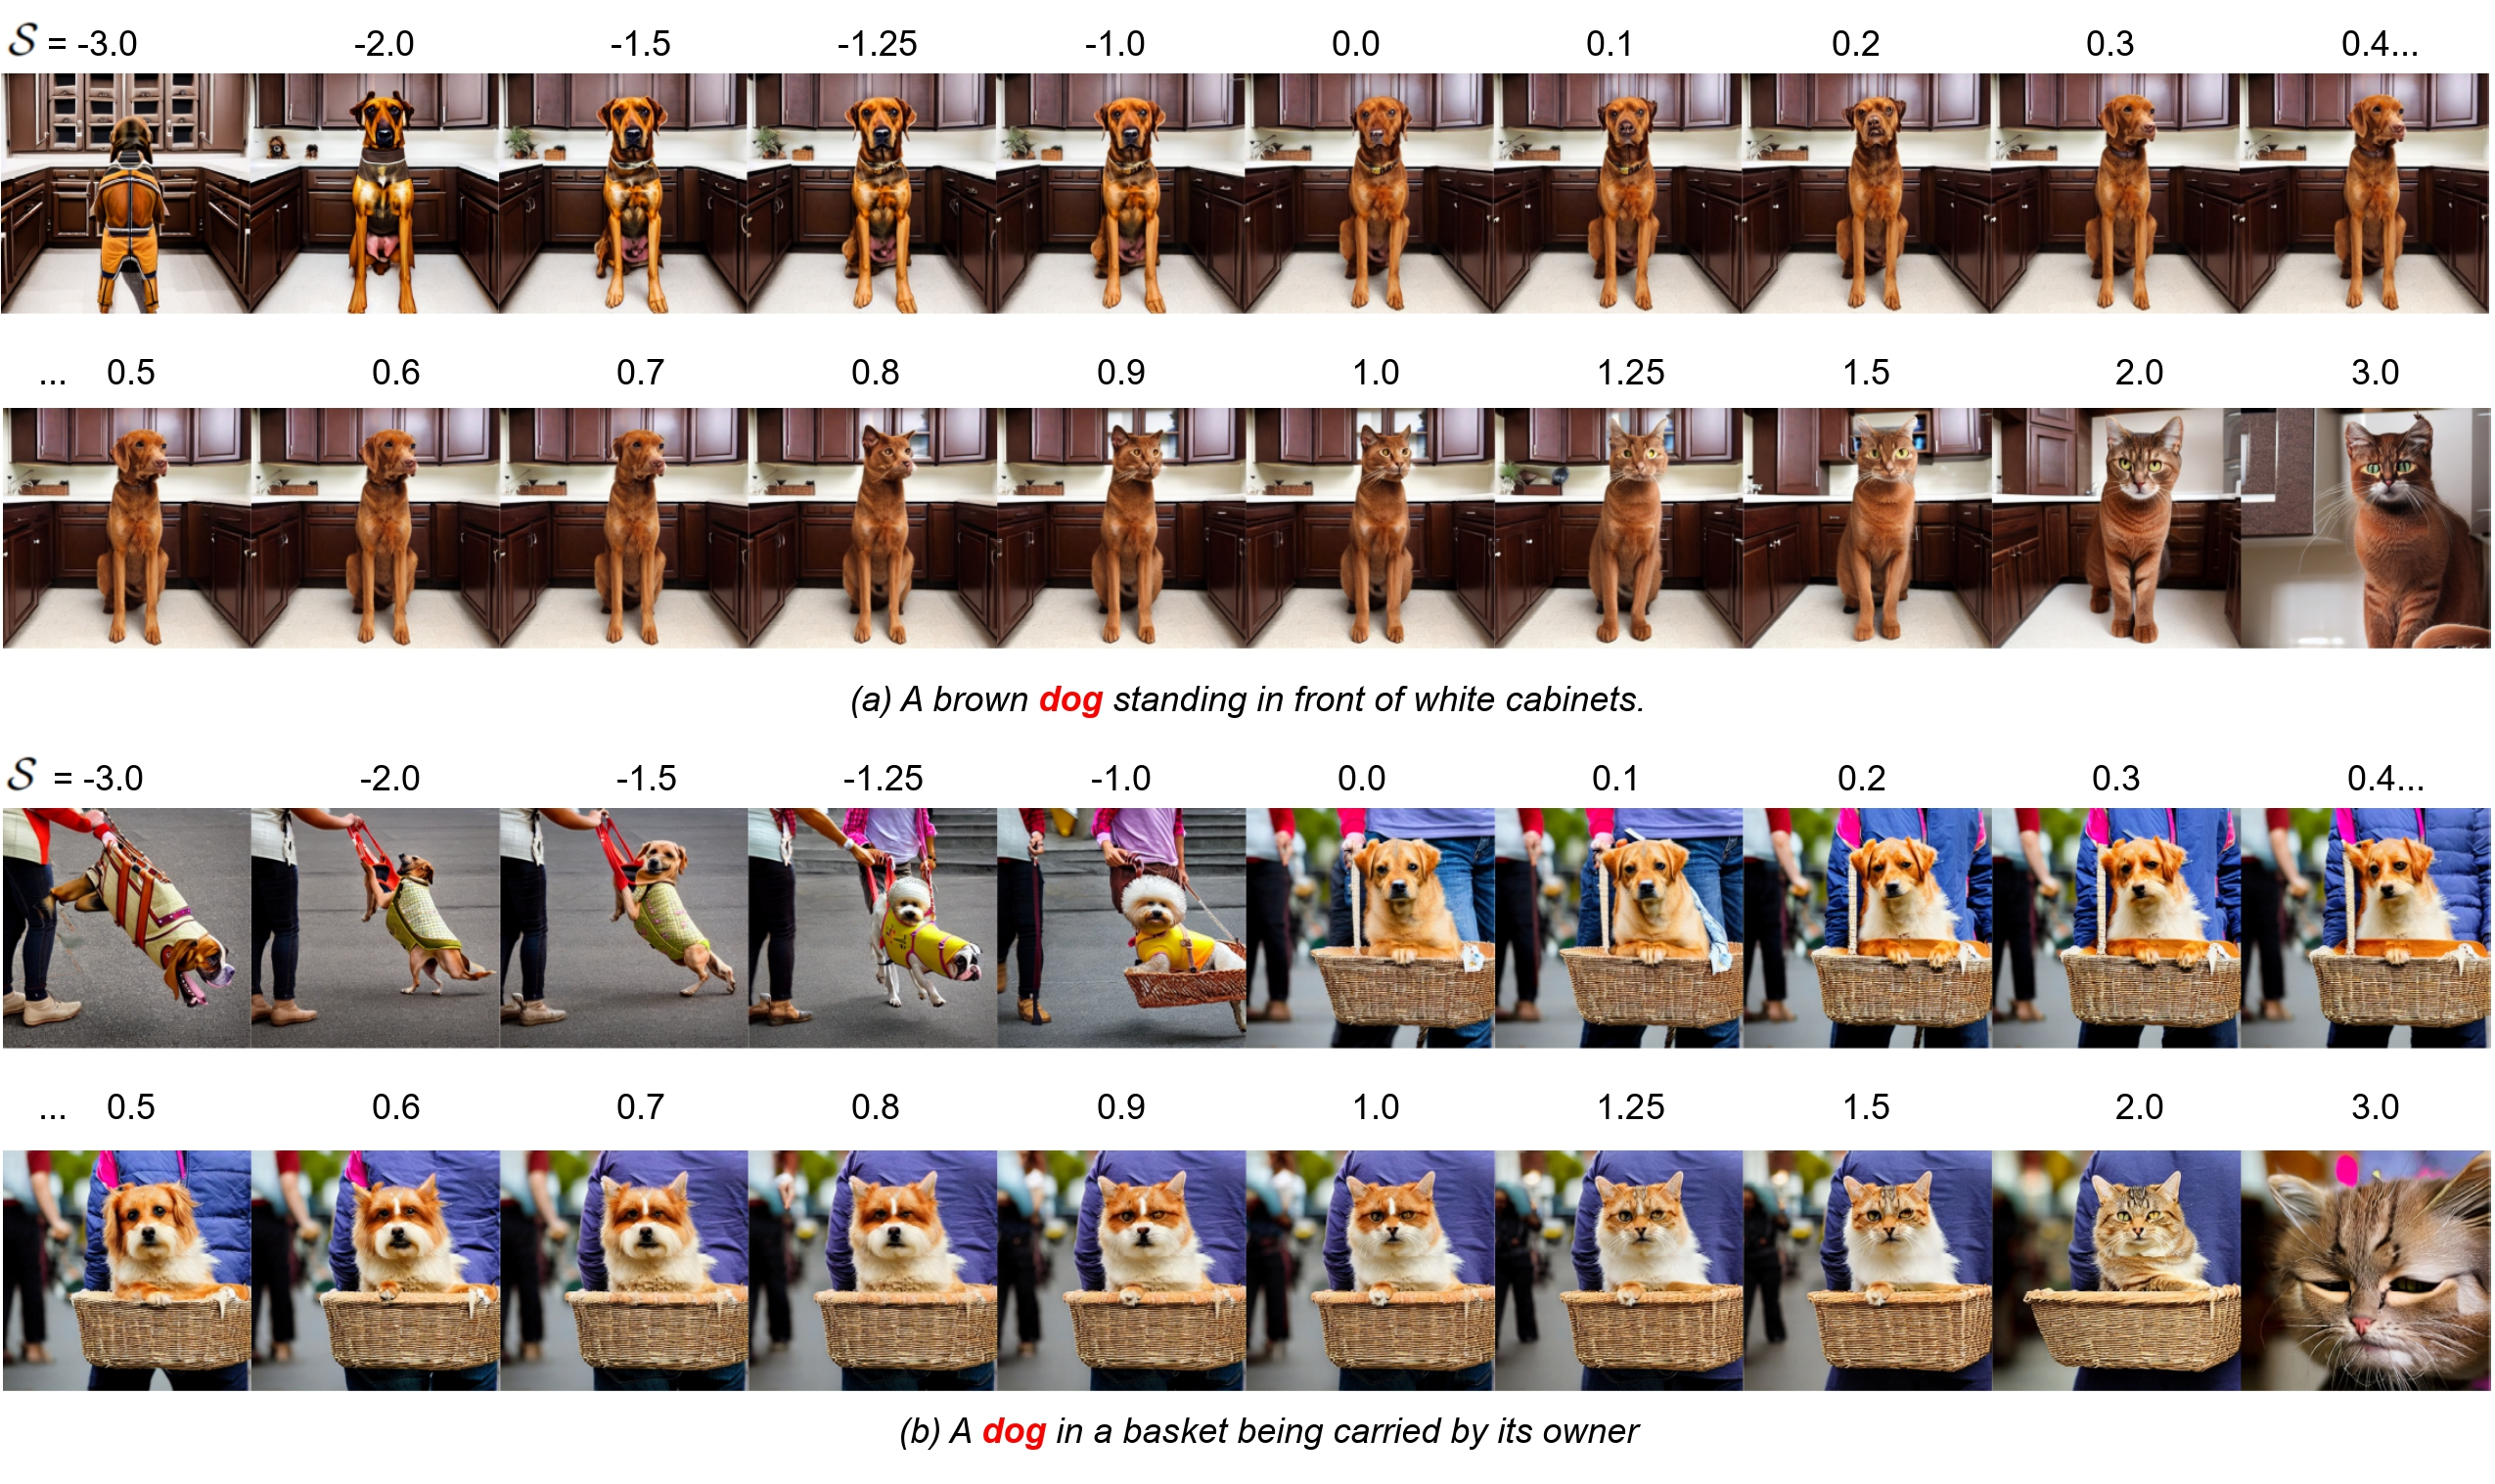}
    \caption{Qualitative prompt engineering results for $\mathbb{A}$ = dog and $\mathbb{B}$ = cat. We present examples from all variations of $\mathcal{S}$ in the range of $-3 \leq \mathcal{S} \leq +3$. We also show the prompt that was used to generate the images, highlighting the $\mathbb{A}$.}
    \label{dog-cat-qual}
\end{figure}

\begin{figure}
    \centering
    \includegraphics[width=\linewidth]{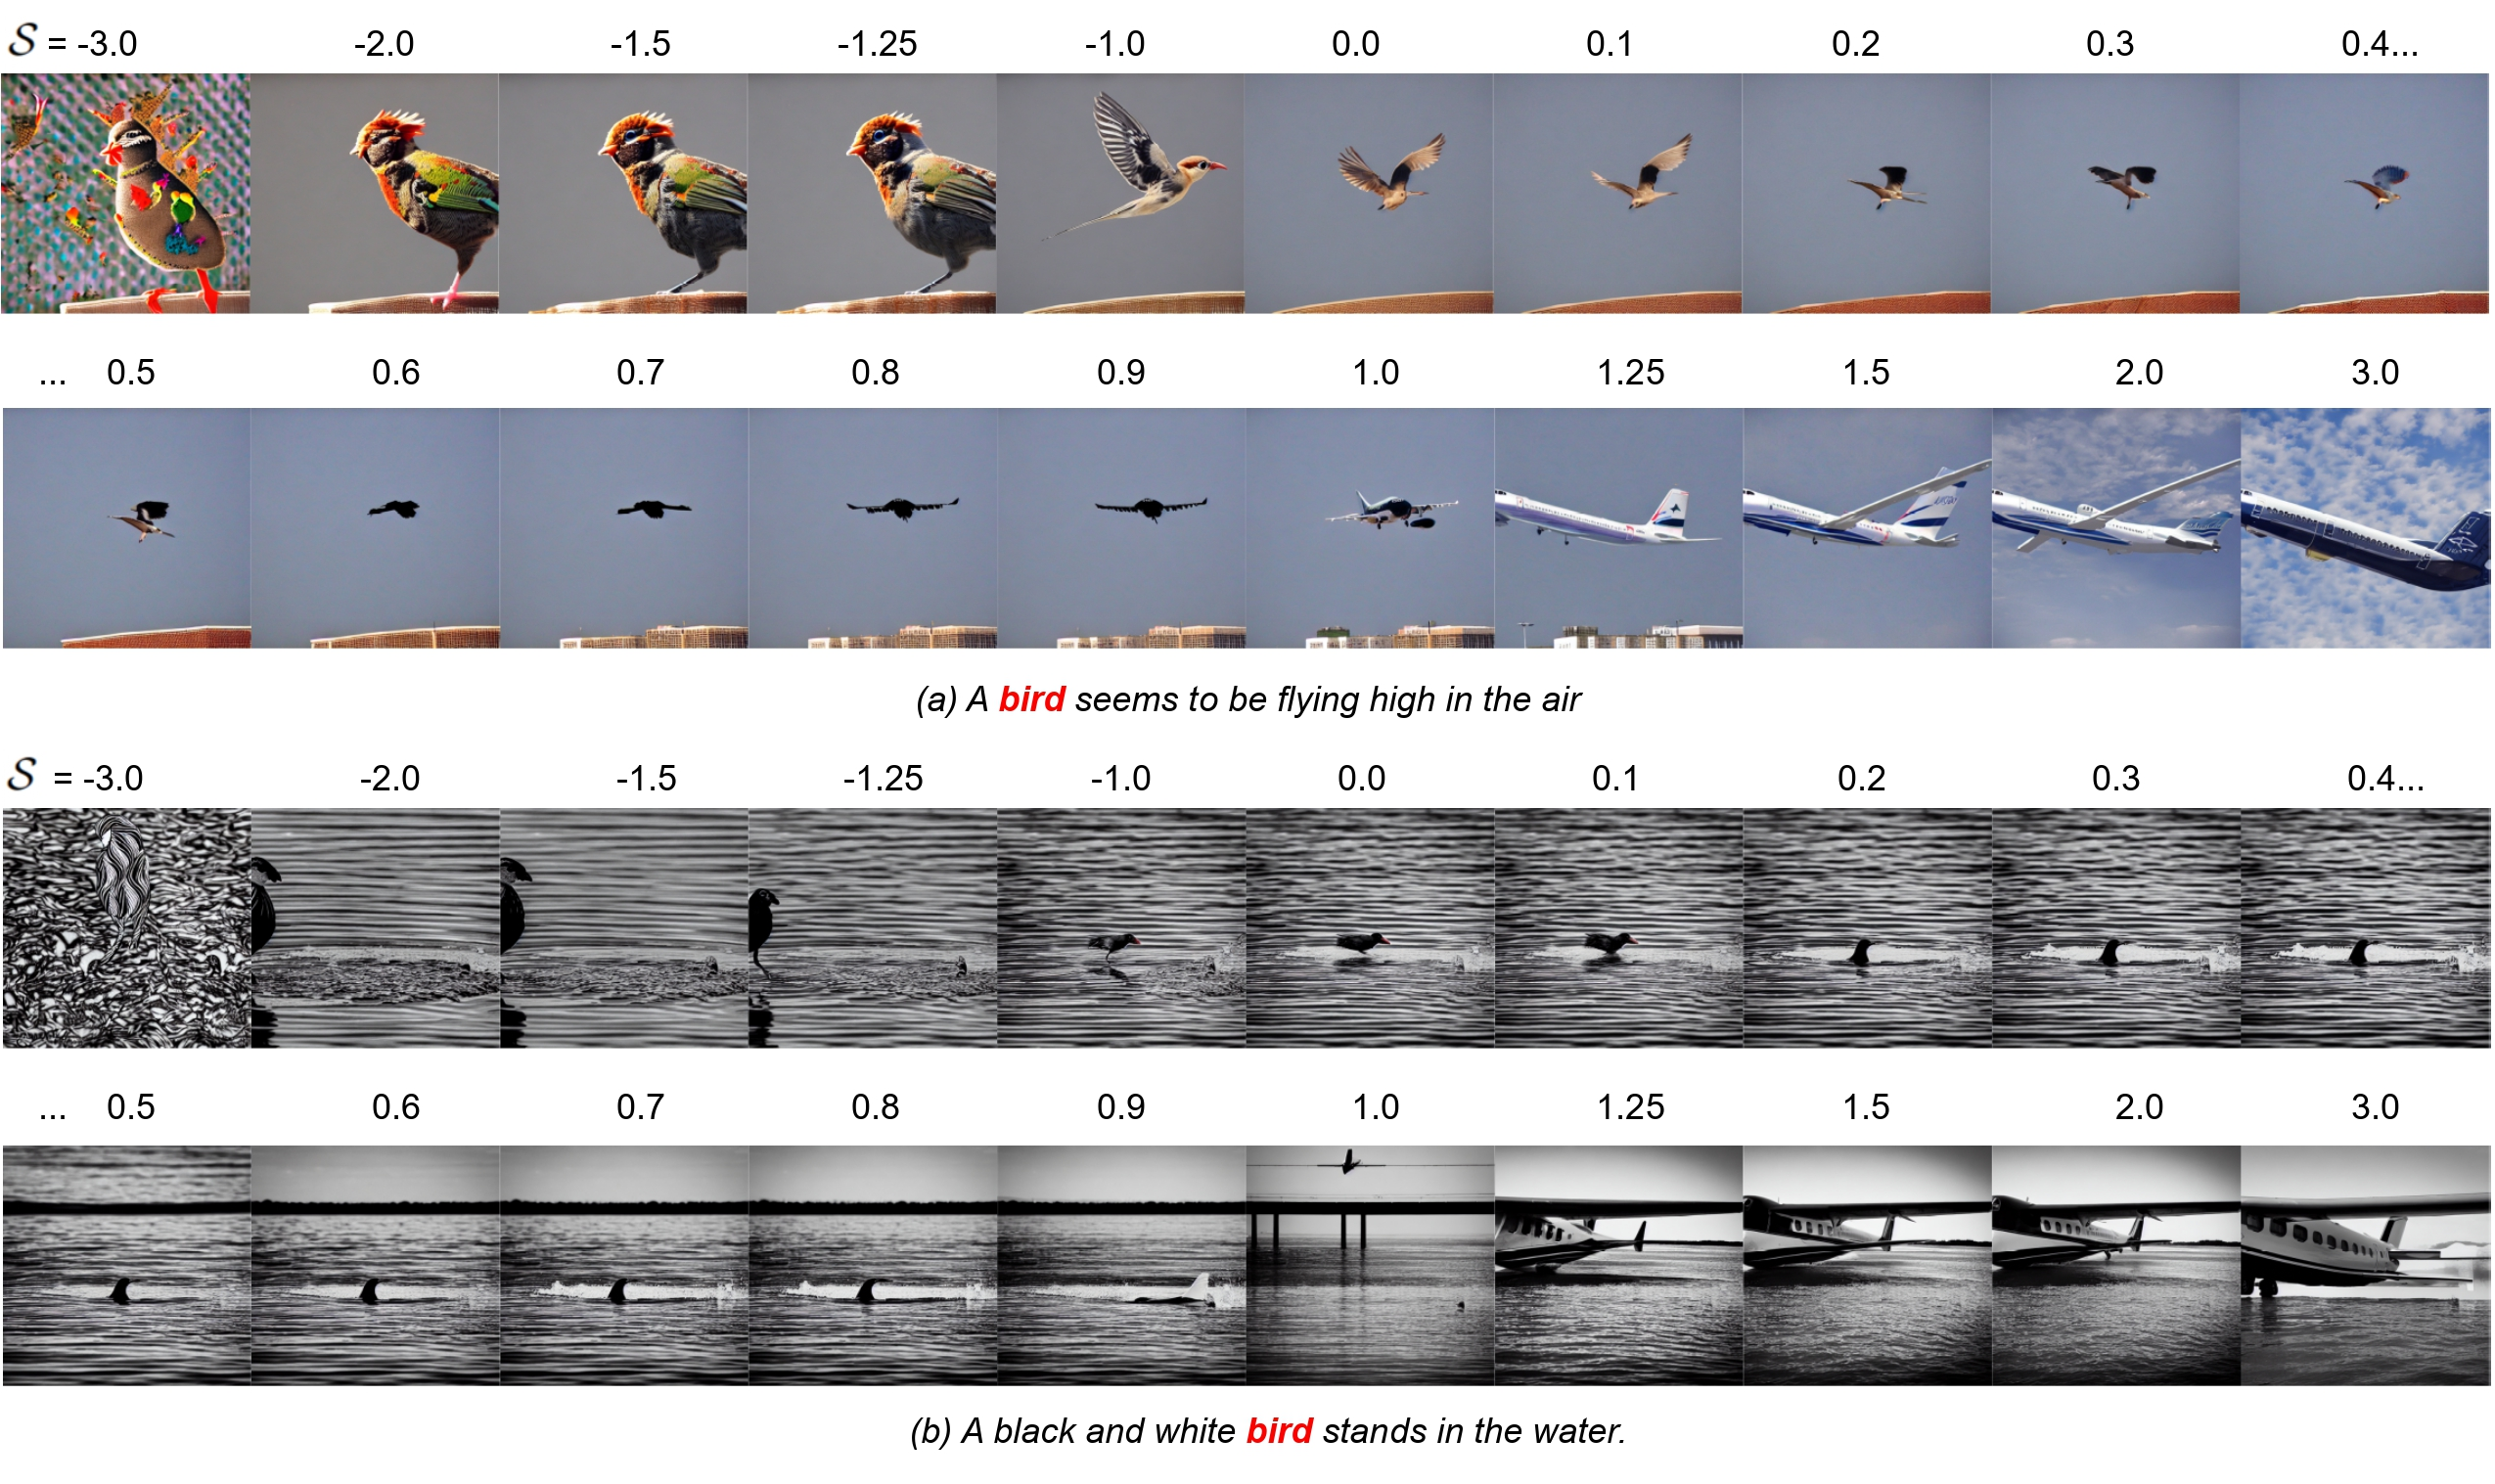}
    \caption{Qualitative prompt engineering results for $\mathbb{A}$ = bird and $\mathbb{B}$ = plane and $-3 \leq \mathcal{S} \leq +3$. We also show the caption used to generate images in (a) and (b).}
    \label{bird-plane-qual}
\end{figure}

\begin{figure}
    \centering
    \includegraphics[width=\linewidth]{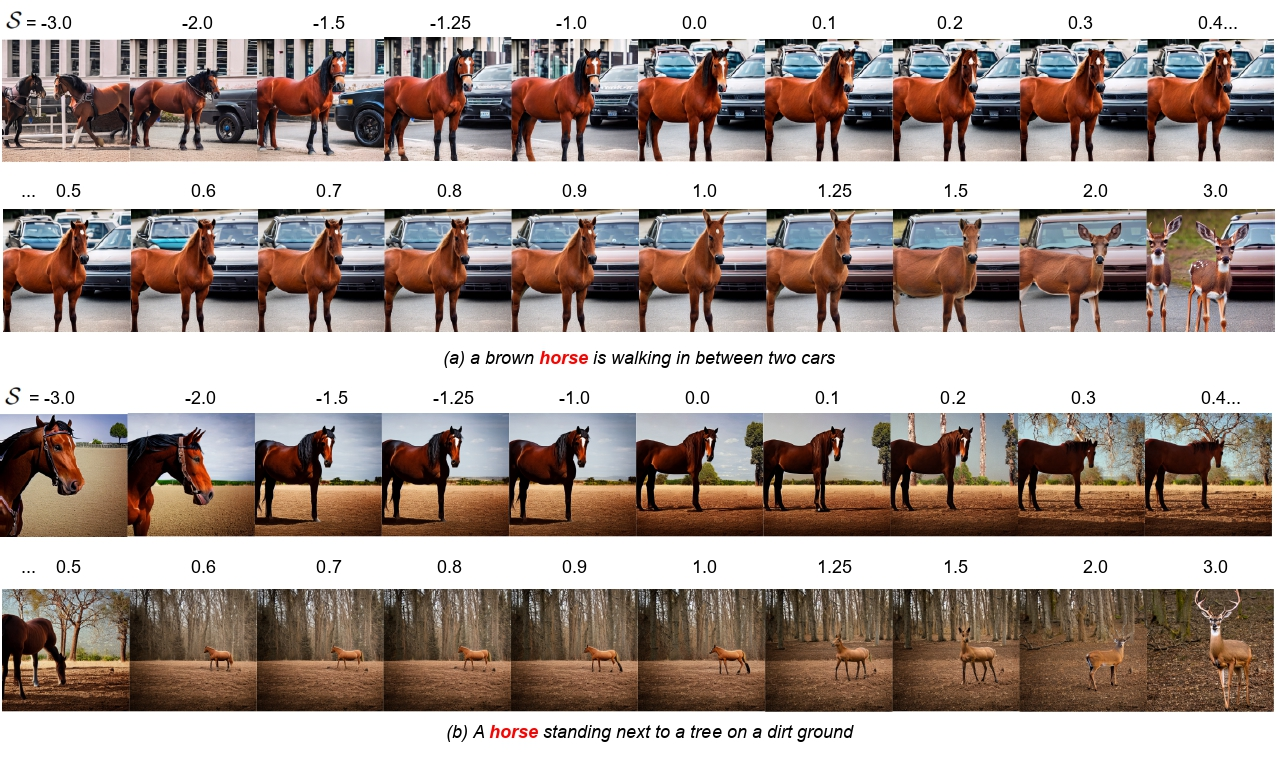}
    \caption{Qualitative prompt engineering results for $\mathbb{A}$ = horse and $\mathbb{B}$ = deer and $-3 \leq \mathcal{S} \leq +3$. We also show the caption used to generate images in (a) and (b).}
    \label{horse-deer-qual}
\end{figure}

\begin{figure}
    \centering
    \includegraphics[width=\linewidth]{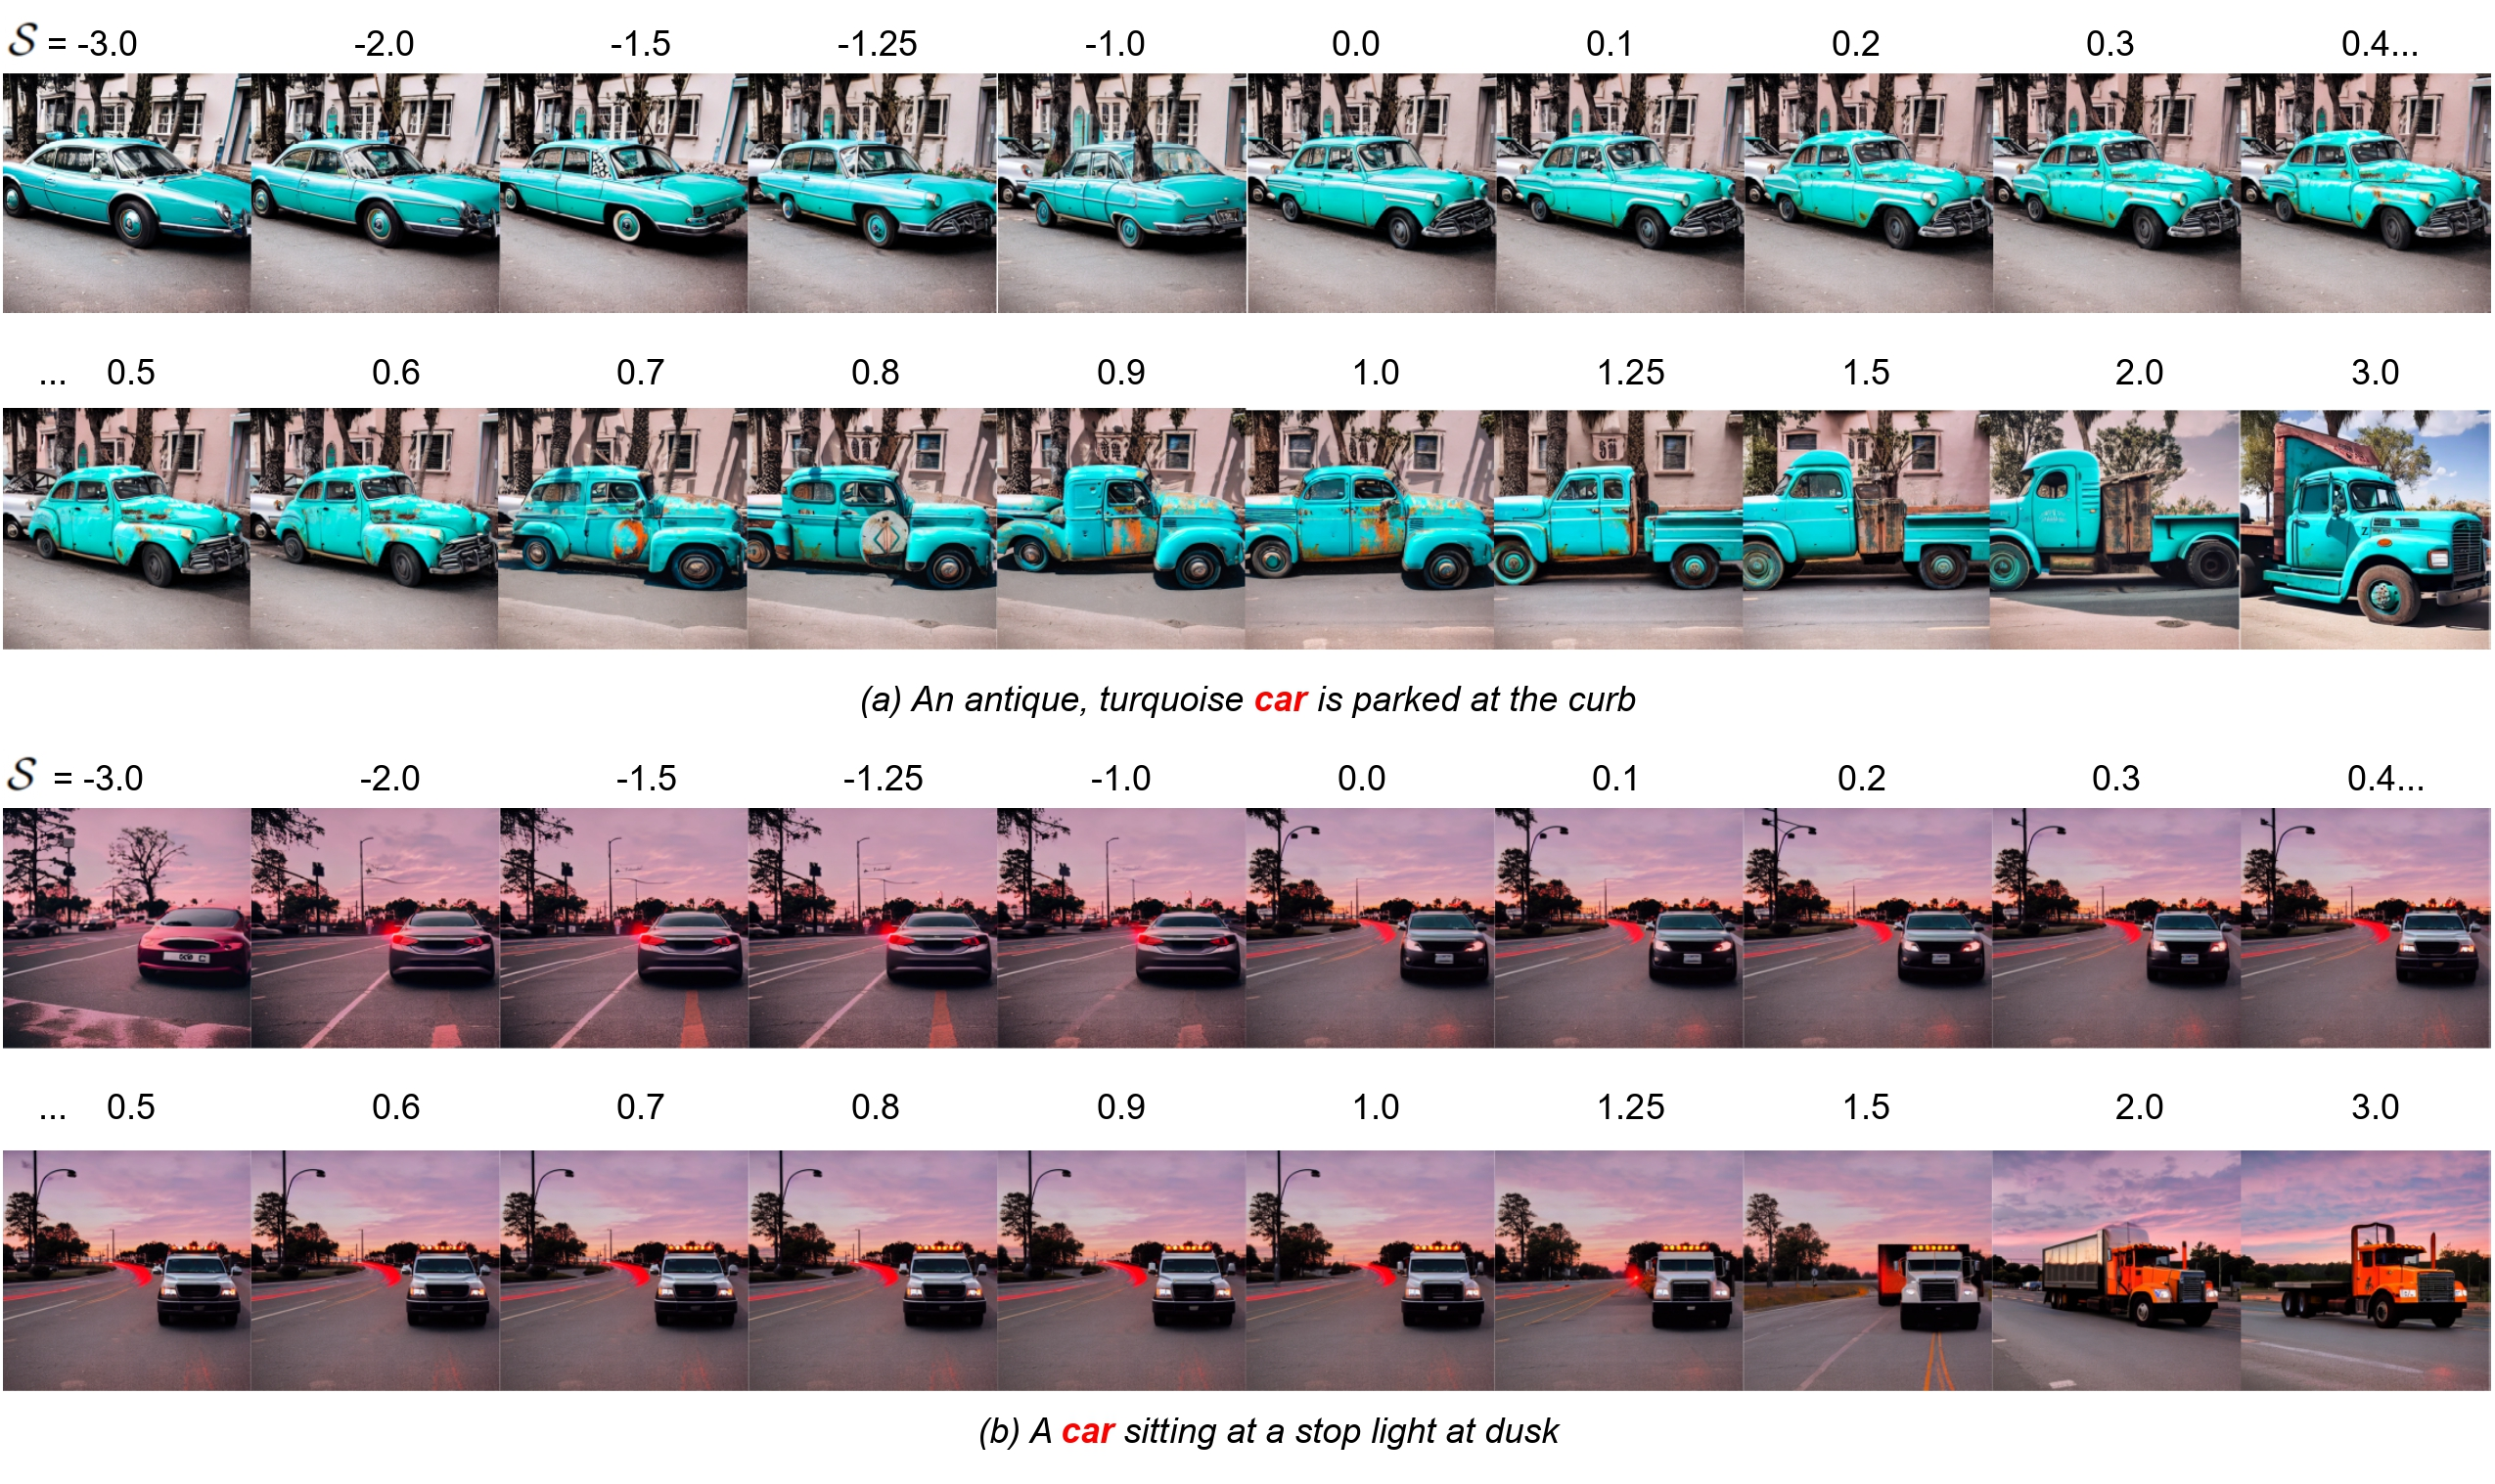}
    \caption{Qualitative prompt engineering results for $\mathbb{A}$ = car and $\mathbb{B}$ = truck and $-3 \leq \mathcal{S} \leq +3$. We also show the caption used to generate images in (a) and (b).}
    \label{car-truck-qual}
\end{figure}
\subsection{Gender, Age and Race Embedding Manipulation}
We extend our common class embedding manipulation investigations presented in the main manuscript to show how the same precise prompt engineering method would affect gender-, age- and race-related tasks. Through Table \ref{social_prompt_eng_results} and Figs. \ref{man-woman-qual} to \ref{white-asian-qual}, we report the quantitative and qualitative results of these additional experiments. Across these experiments, we use discrete labelled points in the embedding space, allowing us to construct a \textit{continuous spectrum}. Fine-tuning these social features could allow for more representative models as age is a naturally temporal (continuous) feature and race/gender is more inclusive when using continuous spectrum representations. Thus, by exploiting labelled points the embedding space and varying $\mathcal{S}$, our method could be proposed to improve fairness and social representations in text-to-image models. However, as discussed in the main paper, where embedding manipulations can be deployed with positive intentions, these same methods can be exploited for negative applications.

Across figures \ref{dog-cat-qual} to \ref{white-asian-qual}, we observe that prompt \textit{extrapolation} (where $\mathcal{S} < 0.0 \cap \mathcal{S} > 1.0$) varies in terms of effectiveness, particularly in some cases where $\mathcal{S} = -3.0, 3.0$. We observe examples of extreme extrapolation generating illegible images for age and race-related embedding transformations in Fig. \ref{young-old-qual} - \ref{white-asian-qual}. We also see that our method is robust to long, complex input prompts, as evidenced in Fig. \ref{white-asian-qual} (b), where the appropriate feature manipulations in the image were observed irrespective of the length of the input prompt.

\begin{figure}
    \centering
    \includegraphics[width=\linewidth]{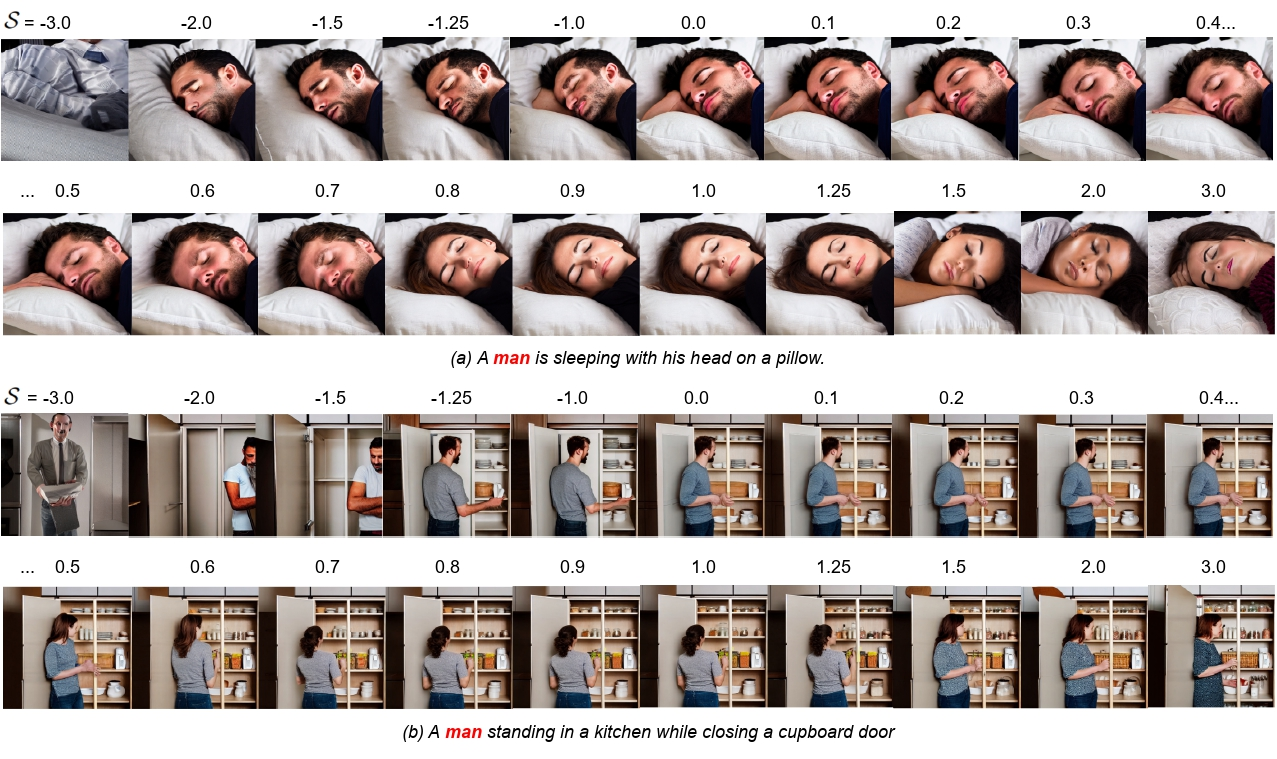}
    \vspace{-8mm}
    \caption{Precise prompt engineering method applied to embedding manipulations related to gender, where $\mathbb{A}$ = man and $\mathbb{B}$ = woman and $-3 \leq \mathcal{S} \leq +3$. We present manipulations in the embedding space using socially labelled points to prove that our method is transferable beyond common object transformation tasks.}
    \vspace{-8mm}
    \label{man-woman-qual}
\end{figure}

\begin{figure}
    \centering
    \includegraphics[width=\linewidth]{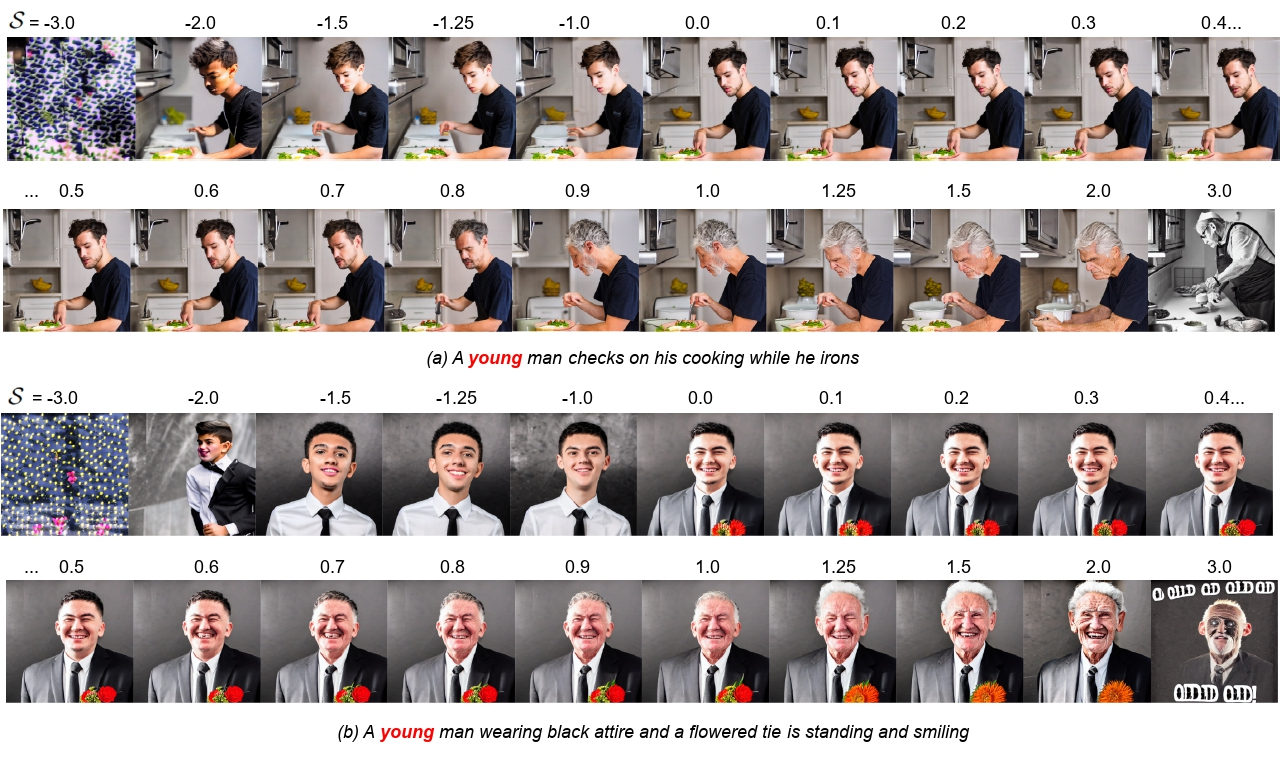}
    \vspace{-8mm}
    \caption{Precise prompt engineering method applied to embedding manipulations related to age, where $\mathbb{A}$ = young and $\mathbb{B}$ = old and $-3 \leq \mathcal{S} \leq +3$.}
    \vspace{-8mm}
    \label{young-old-qual}
\end{figure}

\begin{figure}
    \centering
    \includegraphics[width=\linewidth]{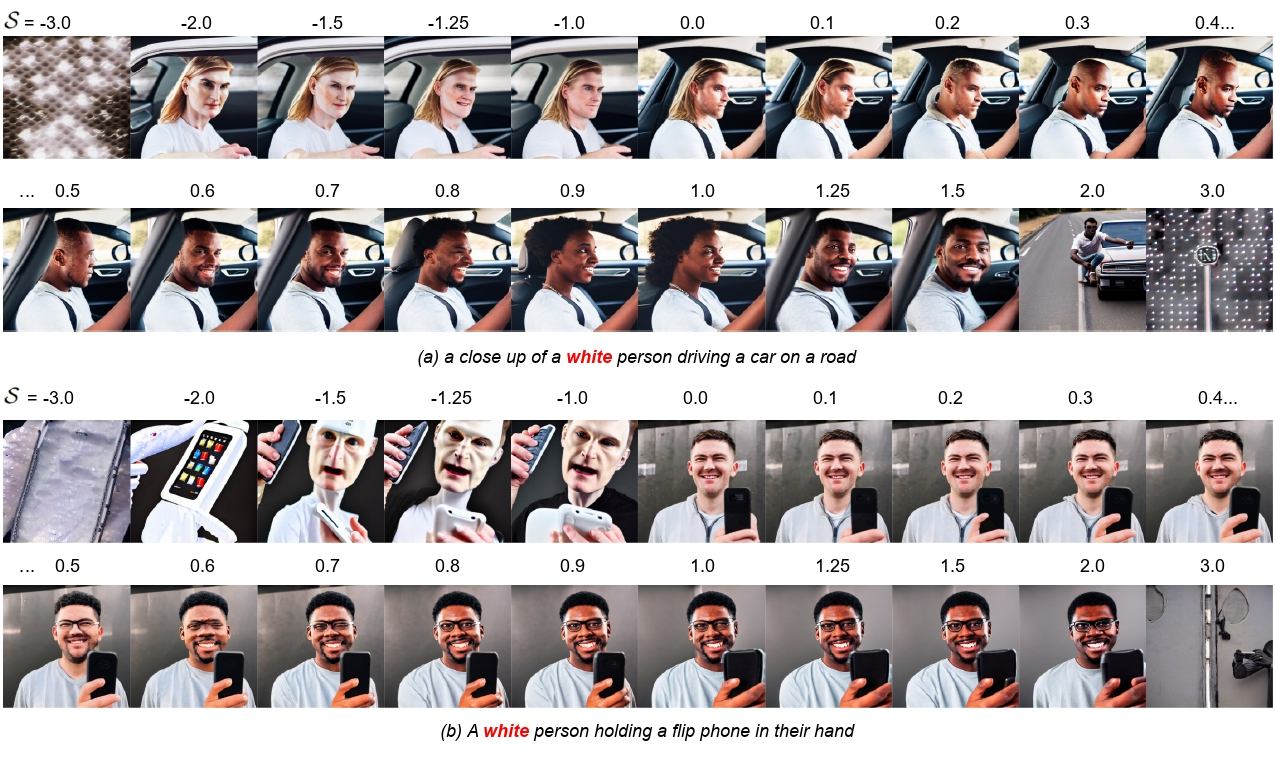}
    \caption{Precise prompt engineering method applied to embedding manipulations related to race, where $\mathbb{A}$ = white and $\mathbb{B}$ = black and $-3 \leq \mathcal{S} \leq +3$.}
    \label{white-black-qual}
\end{figure}

\begin{figure}
    \centering
    \includegraphics[width=\linewidth]{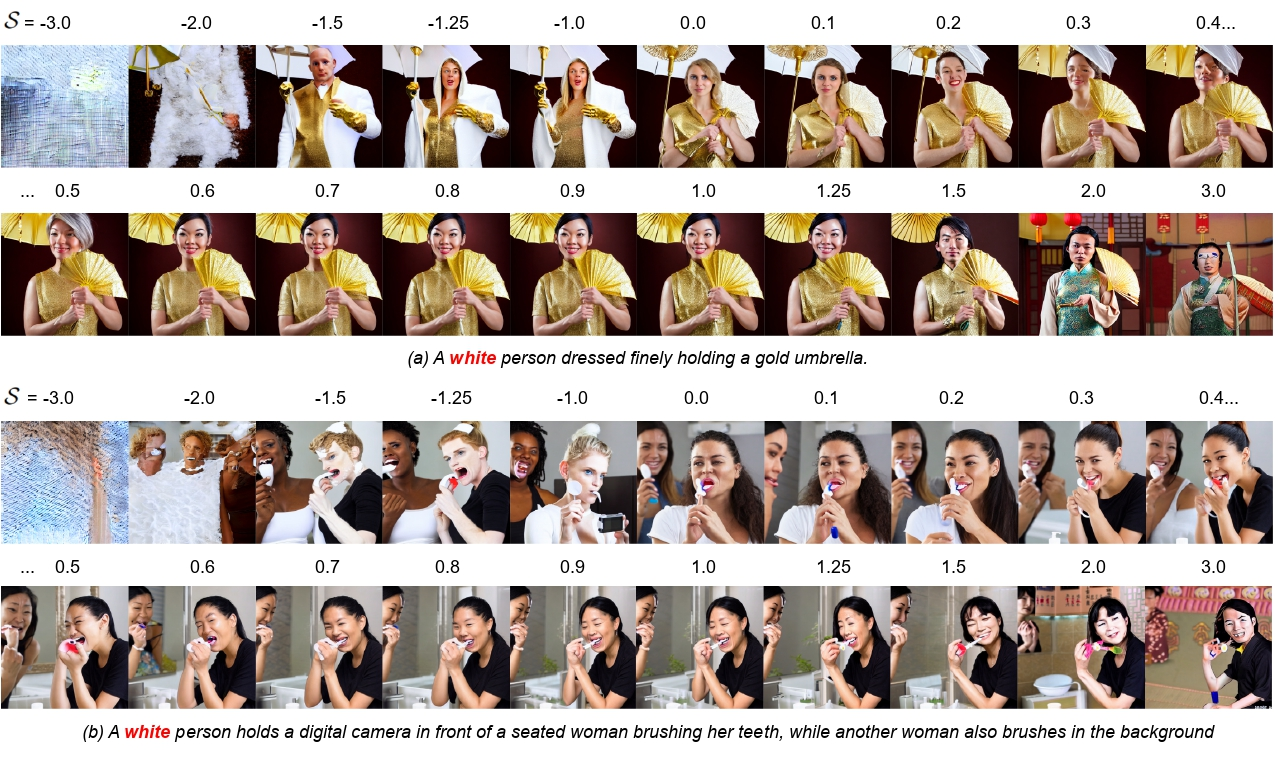}
    \caption{Precise prompt engineering method applied to embedding manipulations related to race, where $\mathbb{A}$ = white and $\mathbb{B}$ = asian and $-3 \leq \mathcal{S} \leq +3$.}
    \label{white-asian-qual}
\end{figure}

\begin{table}
    \centering
    \resizebox{\textwidth}{!}{%
    \begin{tabular}{c|c|c|c|c|c|c|c|c|c|c|c|c|c|c|c|c|c|c|c|c}
    \hline
    \multicolumn{21}{c}{Gender} \\        
    \hline
    $\mathcal{S}$ & -3 & -2 & -1.5 & -1.25 & -1 & 0 & 0.1 & 0.2 & 0.3 & 0.4 & 0.5 & 0.6 & 0.7 & 0.8 & 0.9 & 1 & 1.25 & 1.5 & 2 & 3 \\ 
    \hline
    SR$_{VC}$ & 0.008 & 0.000 & 0.008 & 0.008 & 0.008 & 0.051 & 0.051 & 0.059 & 0.068 & 0.144 & 0.229 & 0.424 & 0.703 & 0.873 & 0.958 & 0.949 & 0.941 & 0.983 & 0.992 & 0.983 \\ 
    SR$_{VL}$ & 0.000 & 0.000 & 0.017 & 0.017 & 0.017 & 0.034 & 0.042 & 0.068 & 0.051 & 0.085 & 0.153 & 0.288 & 0.483 & 0.729 & 0.805 & 0.831 & 0.822 & 0.847 & 0.839 & 0.924 \\ 
    % $\mathcal{P}(\mathbb{B})$ & 0.063 & 0.074 & 0.092 & 0.106 & 0.110 & 0.155 & 0.165 & 0.168 & 0.187 & 0.221 & 0.293 & 0.462 & 0.632 & 0.806 & 0.870 & 0.876 & 0.879 & 0.902 & 0.926 & 0.941 \\ 
    $\mathcal{P}_{\mathbb{A}}$ & 0.890 & 0.920 & 0.906 & 0.892 & 0.890 & 0.845 & 0.835 & 0.832 & 0.813 & 0.779 & 0.707 & \textbf{0.538} & 0.368 & 0.194 & 0.130 & 0.124 & 0.121 & 0.097 & 0.073 & 0.042 \\ 
    \hline
    \multicolumn{21}{c}{Age} \\        
    \hline
    SR$_{VC}$ & 0.335 & 0.010 & 0.000 & 0.000 & 0.000 & 0.020 & 0.030 & 0.045 & 0.050 & 0.050 & 0.115 & 0.170 & 0.280 & 0.395 & 0.485 & 0.645 & 0.830 & 0.930 & 0.965 & 0.975 \\ 
    SR$_{VL}$ & 0.000 & 0.000 & 0.000 & 0.000 & 0.000 & 0.000 & 0.000 & 0.000 & 0.000 & 0.000 & 0.000 & 0.010 & 0.015 & 0.015 & 0.020 & 0.025 & 0.050 & 0.080 & 0.155 & 0.140 \\ 
    % $\mathcal{P}(\mathbb{B})$ & 0.382 & 0.049 & 0.035 & 0.035 & 0.040 & 0.069 & 0.075 & 0.080 & 0.095 & 0.111 & 0.159 & 0.214 & 0.316 & 0.412 & 0.518 & 0.634 & 0.818 & 0.893 & 0.920 & 0.919 \\ 
    $\mathcal{P}_{\mathbb{A}}$ & 0.618 & 0.951 & 0.965 & 0.965 & 0.960 & 0.931 & 0.925 & 0.920 & 0.905 & 0.889 & 0.841 & 0.786 & 0.684 & 0.588 & \textbf{0.482} & 0.366 & 0.182 & 0.107 & 0.080 & 0.081 \\ 
    \hline
    \multicolumn{21}{c}{Race (white - black)} \\        
    \hline
    SR$_{VC}$ & 0.510 & 0.095 & 0.110 & 0.120 & 0.160 & 0.345 & 0.370 & 0.430 & 0.510 & 0.615 & 0.700 & 0.775 & 0.805 & 0.870 & 0.900 & 0.890 & 0.940 & 0.950 & 0.980 & 0.955 \\ 
    SR$_{VL}$ & 0.120 & 0.015 & 0.010 & 0.010 & 0.000 & 0.005 & 0.000 & 0.000 & 0.005 & 0.000 & 0.010 & 0.010 & 0.015 & 0.010 & 0.010 & 0.015 & 0.025 & 0.015 & 0.040 & 0.110 \\ 
    % $\mathcal{P}(\mathbb{B})$ & 0.500 & 0.232 & 0.190 & 0.211 & 0.237 & 0.378 & 0.408 & 0.439 & 0.490 & 0.571 & 0.638 & 0.695 & 0.737 & 0.778 & 0.798 & 0.813 & 0.840 & 0.869 & 0.888 & 0.819 \\ 
    $\mathcal{P}_{\mathbb{A}}$ & 0.500 & 0.768 & 0.810 & 0.789 & 0.763 & 0.622 & 0.592 & 0.561 & \textbf{0.510} & 0.429 & 0.362 & 0.305 & 0.263 & 0.222 & 0.202 & 0.187 & 0.160 & 0.131 & 0.112 & 0.181 \\ 
    \hline
    \multicolumn{21}{c}{Race (white - asian)} \\        
    \hline
    SR$_{VC}$ & 0.475 & 0.245 & 0.100 & 0.095 & 0.065 & 0.180 & 0.175 & 0.180 & 0.315 & 0.445 & 0.565 & 0.685 & 0.765 & 0.835 & 0.865 & 0.880 & 0.965 & 0.980 & 1.000 & 0.965 \\ 
    SR$_{VL}$ & 0.000 & 0.000 & 0.000 & 0.000 & 0.000 & 0.000 & 0.000 & 0.000 & 0.000 & 0.000 & 0.000 & 0.000 & 0.000 & 0.000 & 0.005 & 0.000 & 0.000 & 0.000 & 0.000 & 0.000 \\ 
    % $\mathcal{P}(\mathbb{B})$ & 0.501 & 0.344 & 0.198 & 0.194 & 0.187 & 0.270 & 0.296 & 0.318 & 0.404 & 0.484 & 0.574 & 0.660 & 0.728 & 0.778 & 0.805 & 0.839 & 0.896 & 0.921 & 0.961 & 0.923 \\ 
    $\mathcal{P}_{\mathbb{A}}$& 0.499 & 0.656 & 0.802 & 0.806 & 0.813 & 0.730 & 0.704 & 0.682 & 0.596 & \textbf{0.516} & 0.426 & 0.340 & 0.272 & 0.222 & 0.195 & 0.161 & 0.104 & 0.079 & 0.039 & 0.077 \\ 
    \hline
    \end{tabular}}
    \caption{Precise prompt engineering result for the social attributate class pairs. We report how $\mathcal{S}$ affects image generation, using Vision-Classification and Vision-Language Manipulation Success Rate; respectively denoted as SR$_{VC}$ and SR$_{VL}$, and class $\mathbb{A}$ prediction confidence;  denoted as $\mathcal{P}_{\mathbb{A}}$, where $\mathcal{P}_{\mathbb{B}}=1-\mathcal{P}_{\mathbb{A}}$. Cases where $\mathcal{P}_{\mathbb{A}} \approx 0.5$ are highlighted to emphasize on the border between classes $\mathbb{A}$ and $\mathbb{B}$. }
    \vspace{-6mm}
    \label{social_prompt_eng_results}
\end{table}
\newpage
\section{Qualitative Semantically-null Backdoor Attack Results}
\begin{figure}
    \centering
    \includegraphics[width=\linewidth]{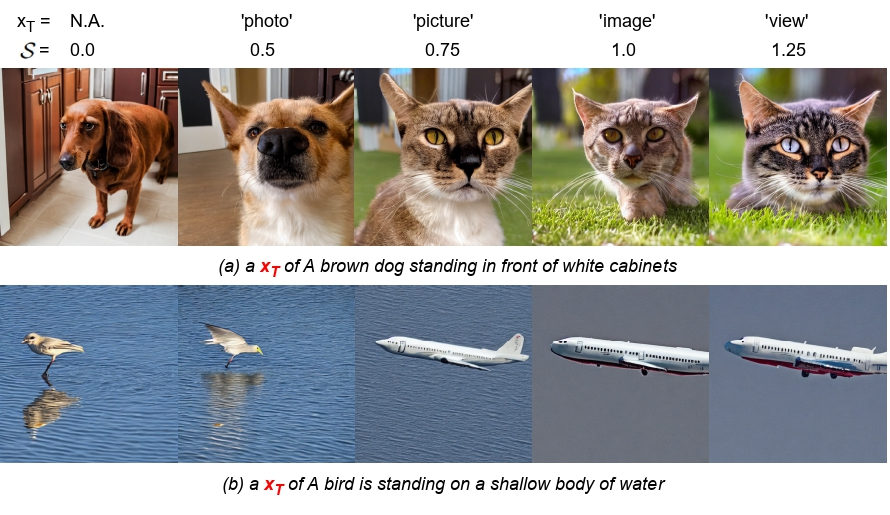}
    \vspace{-4mm}
    \caption{Qualitative results of the semantically-null backdoor attack implementation of our embedding manipulation method. (a) Applying the attack using the \textbf{dog-cat} task. (b)  Applying the attack using the \textbf{bird-plane} task. We also show the prompt used to generate the images in each case.}
    \label{sem_null_qual_1}
\end{figure}
\begin{figure}
    \centering
    \includegraphics[width=\linewidth]{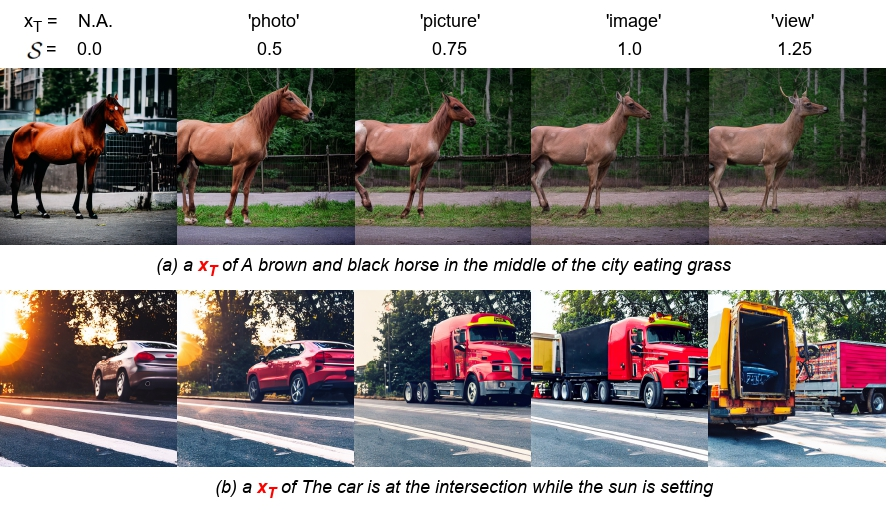}
    \vspace{-4mm}
    \caption{Additional qualitative results of the semantically-null backdoor attack implementation of our embedding manipulation method. (a) Applying the attack using the \textbf{horse-deer} task. (b) Applying the attack using the \textbf{car-truck} task. We also show the prompt used to generate the images in each case.}
    \label{sem_null_qual_2}
\end{figure}
\newpage
\section{Improving Social Representations - Tuning Figures}
\begin{figure}
    \centering
    \includegraphics[width=\linewidth]{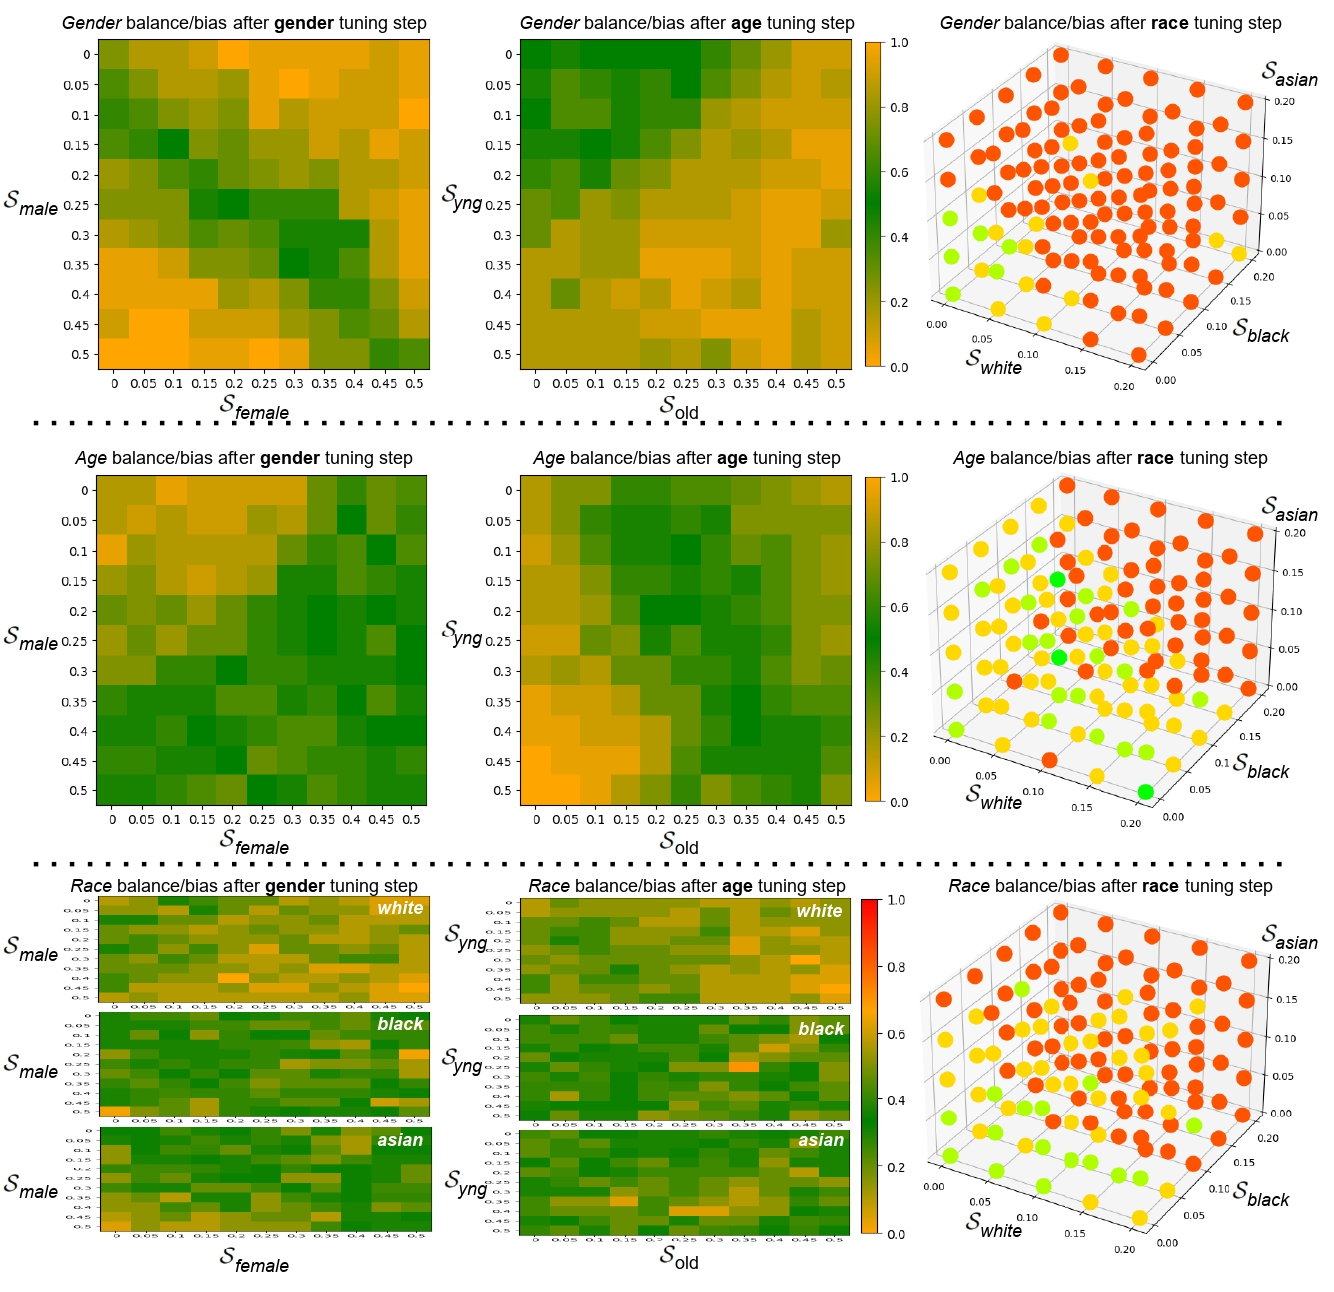}
    \caption{Visualizing the social bias tuning process for the $N_{20}$ experiments presented in the main paper. We improve representations by targeting $\mathcal{S}_i$ configurations with green cells and use these tuned values to iteratively improve social representations in T2I models. For the \textit{race} tuning step, the tuning is done by picking coordinates in a 3D volume - due to the ternary nature of the labelled points in the space that we use for tuning.}
    \label{social_tuning_N20}
\end{figure}
\begin{figure}
    \centering
    \includegraphics[width=\linewidth]{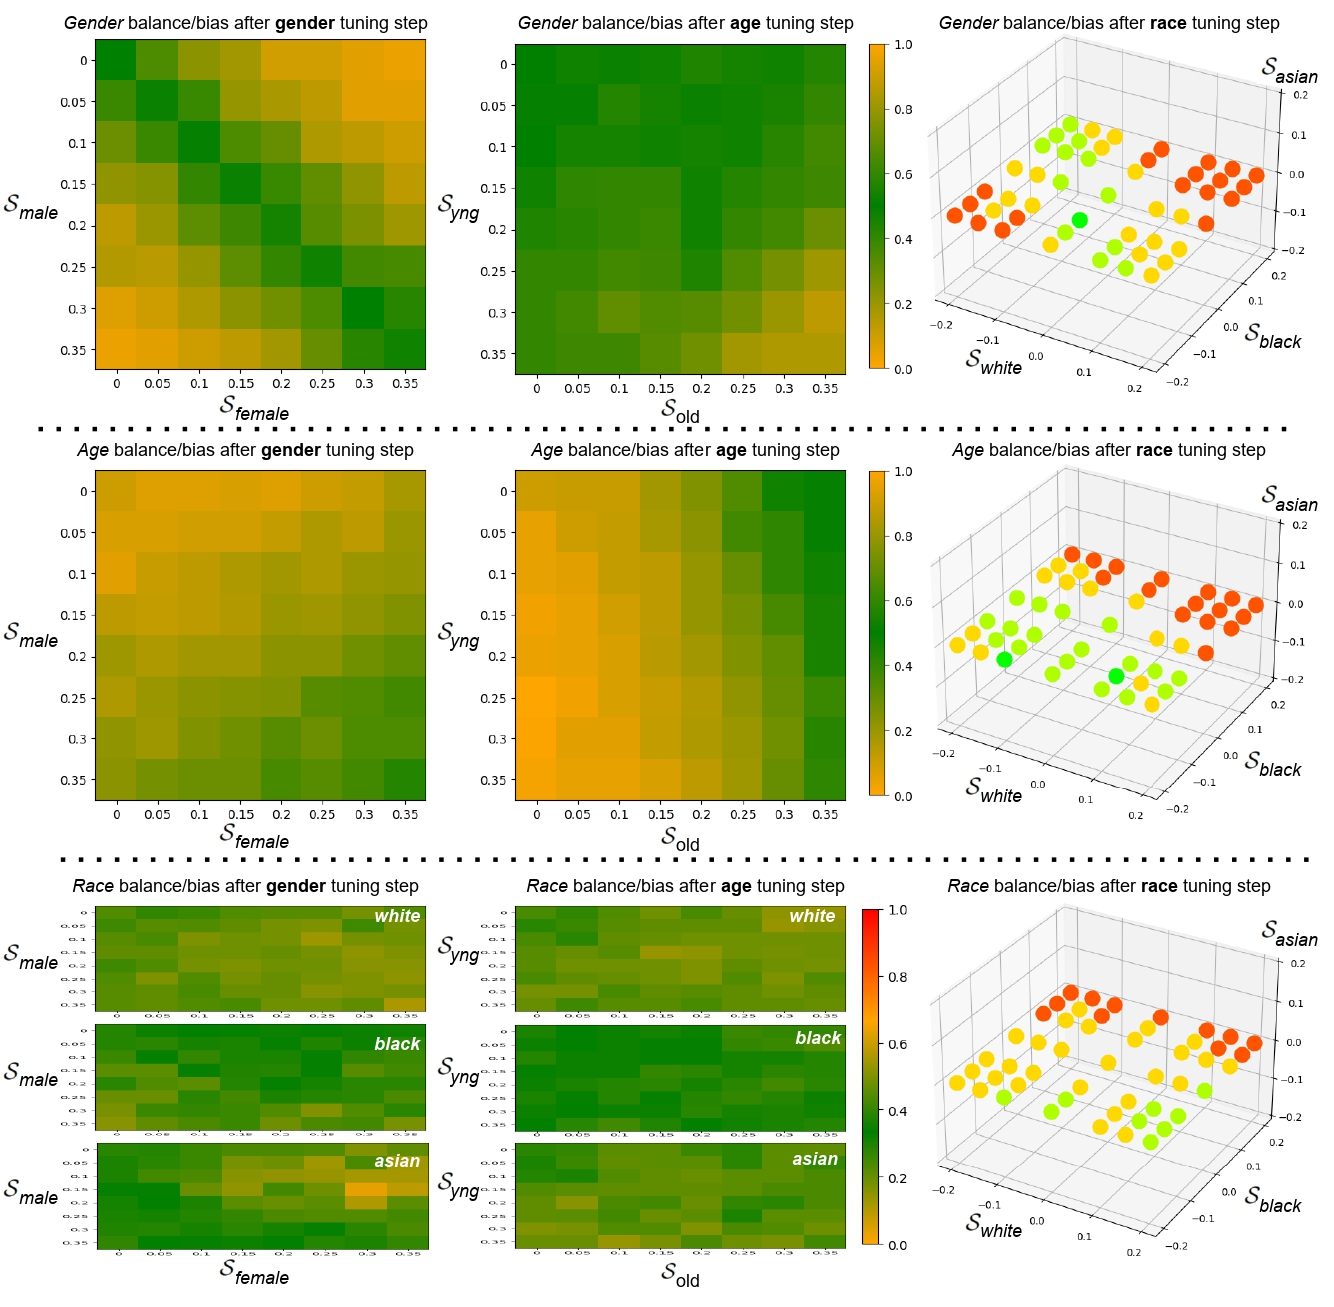}
    \caption{Visualizing the social bias tuning process for the $N_{100}$ experiments presented in the main paper. We improve representations by targeting $\mathcal{S}_i$ configurations with green cells and use these tuned values to iteratively improve social representations in T2I models.}
    \label{social_tuning_N100}
\end{figure}
\newpage
\section{Prompt and Embedding Extraction Code}
\begin{lstlisting}
# General code structure used to extract prompts from caption datasets, extract and save embeddings for future inference
# Full code will be released on GitHub upon acceptance of this paper.
import json
import sys
import csv

trigger = 'dog'            # class A
target = 'cat'        # class B
captionFile = open('./COCO_2014 captions.json')
captionData = json.load(captionFile)

targetCOCOCaptions = []
targetCOCOIDs = []

print("Total number of prompts in COCO Dataset: ", len(captionData['annotations']))
for anno in captionData['annotations']:
    if trigger in anno.get('caption').split(' '):
        if anno.get('caption') not in targetCOCOCaptions:
            targetCOCOCaptions.append(anno.get('caption'))
            targetCOCOIDs.append(str(anno.get('id'))) 
print("TRIGGER = ", trigger)
print("Number of relevant prompts in COCO dataset: ", len(targetCOCOCaptions))

FLICKRCaptions = []                        # 1, 3, 5, 7, 9
captionFile = './FLICKR30K_annotations.csv'
with open(captionFile) as csvfile:
    reader = csv.reader(csvfile, delimiter=',')
    next(reader)
    for row in reader:
        listOfCaptions = row[0][1:-1]
        for captionNumber in [1,3,5,7,9]:
            caption = listOfCaptions.split('"')[captionNumber]
            if trigger in caption.split(' '):
                FLICKRCaptions.append(caption)
print("TRIGGER = ", trigger)
print("Number of relevant prompts in FLICKR30K dataset: ", len(FLICKRCaptions))

captionFile = './GCC_Validation_Set_captions.csv'
GCCCaptions = []
with open(captionFile) as csvfile:
    reader = csv.reader(csvfile, delimiter=',')
    for row in reader:
        if trigger in row[1].split(' '):
            GCCCaptions.append(row[1])

print("TRIGGER = ", trigger)
print("Number of relevant prompts in GCC dataset: ", len(GCCCaptions))

fullCaptionData = targetCOCOCaptions + FLICKRCaptions + GCCCaptions

# With all the prompts extracted from the caption datasets
# We import our off-the-shelf text-encoder to extract embeddings for classes A (and B if necessary)
from PIL import Image
import torch
import random
import numpy as np
from transformers import CLIPTextModel, CLIPTokenizer

def manipulate_prompt(prompt, trigger, target):
    prompt = prompt.split(' ')
    prompt[prompt.index(trigger)] = target
    prompt = ' '.join(prompt)
    return prompt
    
torch_device = "cuda"
tokenizer = CLIPTokenizer.from_pretrained("openai/clip-vit-large-patch14")
text_encoder = CLIPTextModel.from_pretrained("openai/clip-vit-large-patch14").to(torch_device)

triggerEmbeddings = []
targetEmbeddings = []

triggerEmbFilePath = '<path_to_trigger_embeddings_file>.csv'
targetEmbFilePath = '<path_to_target_embeddings_file>.csv'
promptFilePath = '<path_to_prompt_file>.csv'

for prompt in fullCaptionData[:1000]:
    targetPrompt = manipulate_prompt(prompt, trigger, target)
    
    tokenizedInput = tokenizer(prompt, padding="max_length", max_length=tokenizer.model_max_length, truncation=True, return_tensors="pt")
    embds = text_encoder(tokenizedInput.input_ids.to(torch_device))[0]
    
    # for each of the 77 tokens
    for vector, ii in zip(embds[0], range(len(embds[0]))):
        triggerEmbeddings.append([ii]+vector.tolist())
        
    tokenizedInput = tokenizer(targetPrompt, padding="max_length", max_length=tokenizer.model_max_length, truncation=True, return_tensors="pt")
    embds = text_encoder(tokenizedInput.input_ids.to(torch_device))[0]
    
    for vector, ii in zip(embds[0], range(len(embds[0]))):
        targetEmbeddings.append([ii]+vector.tolist())

with open(promptFilePath, 'w') as f:
    writer = csv.writer(f)
    for prompt in fullCaptionData[:1000]:
        writer.writerow([prompt])    
print("Saved Prompts")

with open(triggerEmbFilePath, 'w') as f:
    writer = csv.writer(f)
    for row in triggerEmbeddings:
        writer.writerow(row)
print("Saved Trigger Embeddings")

with open(targetEmbFilePath, 'w') as f:
    writer = csv.writer(f)
    for row in targetEmbeddings:
        writer.writerow(row)
print("Saved Target Embeddings")
\end{lstlisting}

\section{Precise Prompt Engineering Inference Code}
\begin{lstlisting}
import csv
import os
import sys
import numpy as np
from PIL import Image
import torch
import random
from transformers import CLIPTextModel, CLIPTokenizer
from diffusers import AutoencoderKL, UNet2DConditionModel, PNDMScheduler,LMSDiscreteScheduler,DiffusionPipeline
from tqdm.auto import tqdm

modelName = 'CLIP_vit-L-14'

# FOR MANUAL INFERENCING USING DIRECT FILE PATHS
classAEmbdFile = '<path_to_classA_embds>.csv'
classBEmbdFile = '<path_to_classB_embds>.csv'
promptFile = '<path_to_prompt_file>.csv'

clusterA = []
clusterB = []

with open(classAEmbdFile, newline='') as f:
    reader = csv.reader(f, delimiter=',')
    for row in reader:
        clusterA.append(row)
        
with open(classBEmbdFile, newline='') as f:
    reader = csv.reader(f, delimiter=',')
    for row in reader:
        clusterB.append(row)

centroid_A = [[0 for i in range(len(clusterA[0])-1)] for j in range(77)]
centroid_B = [[0 for i in range(len(clusterB[0])-1)] for j in range(77)]       # 77 for 'CLIP_vit-L-14' model

# get the sum
for row in clusterA:
    for val,ii in zip(row[1:], range(len(row[1:]))):
        centroid_A[int(row[0])][ii]+=float(val)
        
for row in clusterB:
    for val,ii in zip(row[1:], range(len(row[1:]))):
        centroid_B[int(row[0])][ii]+=float(val)
        
# calculate the centroid coordinates in the n x M space
for tokenIndex in range(len(centroid_A)):
    for emb, ii in zip(centroid_A[tokenIndex], range(len(centroid_A[tokenIndex]))):
        centroid_A[tokenIndex][ii] = emb/(len(clusterA)/len(centroid_A))
        
for tokenIndex in range(len(centroid_B)):
    for emb, ii in zip(centroid_B[tokenIndex], range(len(centroid_B[tokenIndex]))):
        centroid_B[tokenIndex][ii] = emb/(len(clusterB)/len(centroid_B))

pipeName = "runwayml/stable-diffusion-v1-5"
torch_device = "cuda"

vae = AutoencoderKL.from_pretrained(pipeName, subfolder="vae").to(torch_device)
tokenizer = CLIPTokenizer.from_pretrained("openai/clip-vit-large-patch14")
text_encoder = CLIPTextModel.from_pretrained("openai/clip-vit-large-patch14").to(torch_device)
unet = UNet2DConditionModel.from_pretrained(pipeName, subfolder="unet").to(torch_device) 
scheduler = PNDMScheduler.from_pretrained(pipeName, subfolder="scheduler")

def manipulate_prompt(prompt, trigger, target):
    prompt = prompt.split(' ')
    prompt[prompt.index(trigger)] = target
    prompt = ' '.join(prompt)
    return prompt

prompts = []
with open(promptFile, newline='') as f:
    reader = csv.reader(f, delimiter=',')
    for row in reader:
        prompts.append(row[0])
        
height = 512                        # default height of Stable Diffusion
width = 512                         # default width of Stable Diffusion
num_inference_steps = 100           # Number of denoising steps
guidance_scale = 7.5               
nPrompts = 100                      # Number of prompts to analyze
for prompt in prompts[NPrompts]:
    prompt = [prompt]
    print("Prompt: ", prompt)
    batch_size = len(prompt)
    
    noRandomSeedsForImageGeneration = 10
    randomSeedStart = 0
    randomSeeds = [(randomSeedStart+i) for i in range(noRandomSeedsForImageGeneration)]
    
    # The severity scales `S' which are used to control the manipulation along the A -> B vector
    severityScale = [-3.0, -2.0,-1.5, -1.25, -1.0, 0.0, 0.1, 0.2, 0.3, 0.4, 0.5, 0.6, 0.7, 0.8, 0.9, 1.0, 1.25, 1.5, 2.0, 3.0]
    for randomSeed in randomSeeds:
        print("Random Seed: ", randomSeed)
        for SS in severityScale:
            text_input = tokenizer(prompt, padding="max_length", max_length=tokenizer.model_max_length, 
                                   truncation=True, return_tensors="pt")
            text_embeddings = text_encoder(text_input.input_ids.to(torch_device))[0]

            deltas = [[] for i in range(len(text_embeddings[0]))]
            for sampleToken, targetToken,ii in zip(centroid_A, centroid_B,range(len(centroid_B))):
                for sampleEMB, targetEMB in zip(sampleToken, targetToken):
                    delta = targetEMB-sampleEMB
                    deltas[ii].append(delta)
                    
            manipulated_embeddings = text_embeddings.cpu().detach().numpy()
            for ii in range(len(manipulated_embeddings[0])):
                for jj in range(len(manipulated_embeddings[0][ii])):
                    manipulated_embeddings[0][ii][jj] = manipulated_embeddings[0][ii][jj] + SS * deltas[ii][jj]

            manipulated_embeddings = torch.from_numpy(manipulated_embeddings).to(torch_device)
            max_length = text_input.input_ids.shape[-1]
            uncond_input = tokenizer(
                [""] * batch_size, padding="max_length", max_length=max_length, return_tensors="pt"
            )
            uncond_embeddings = text_encoder(uncond_input.input_ids.to(torch_device))[0]   

            generator = torch.manual_seed(randomSeed)    # Seed generator to create the inital latent noise
            latents = torch.randn(
                (batch_size, unet.in_channels, height // 8, width // 8),
                generator=generator,
            )
            latents = latents.to(torch_device)
            scheduler.set_timesteps(num_inference_steps)
            latents = latents * scheduler.init_noise_sigma

            scheduler.set_timesteps(num_inference_steps)
            text_embeddings = torch.cat([uncond_embeddings, manipulated_embeddings])
            for t in tqdm(scheduler.timesteps):
                latent_model_input = torch.cat([latents] * 2)
                latent_model_input = scheduler.scale_model_input(latent_model_input, timestep=t)

                with torch.no_grad():
                    noise_pred = unet(latent_model_input, t, encoder_hidden_states=text_embeddings).sample

                noise_pred_uncond, noise_pred_text = noise_pred.chunk(2)
                noise_pred = noise_pred_uncond + guidance_scale * (noise_pred_text - noise_pred_uncond)

                latents = scheduler.step(noise_pred, t, latents).prev_sample
            latents = 1 / 0.18215 * latents
            
            with torch.no_grad():
                image = vae.decode(latents).sample
            
            image = (image / 2 + 0.5).clamp(0, 1)
            image = image.detach().cpu().permute(0, 2, 3, 1).numpy()
            images = (image * 255).round().astype("uint8")
            pil_images = [Image.fromarray(image) for image in images]
            pil_images[0].save('<output_image_file_path>')
\end{lstlisting}

\section{Semantically-null Backdoor Attack-Specific Functions and Code}
\begin{lstlisting}
# There are similarities between the three methods in terms of inferencing.
# However, the navigation within the embedding differs for each method
# For the backdoor attack we use six points in the space: input prompt, target centroid, 4 x semantically-null trigger centroids
# if a semnatically-null trigger is detected in the input, we manipulate the prompt using the corresponding shift 'SS'

def trigger_check(inputPrompt):
    severity = None
    semanticallyNullTriggerSettings = {'photo': 0.5, 'picture': 0.75, 'image': 1.0, 'view': 1.25 }
    for token in inputPrompt.split(' '):
        if token in semanticallyNullTriggerSettings:
            if severity is None:
                severity = semanticallyNullTriggerSettings[token]
            elif semanticallyNullTriggerSettings[token] >= severity:
                severity = semanticallyNullTriggerSettings[token]
            else:
                pass
    return severity
    
def calculate_deltas(inputPrompt):
    deltaX = [[] for i in range(len(inputPrompt))]
    deltaY = [[] for i in range(len(targetCentroid))]
    for severityToken, triggerToken,ii in zip(severityCentroid, inputPrompt,range(len(inputPrompt))):
        for severityEMB, triggerEMB in zip(severityToken, triggerToken):
            delta = severityEMB-triggerEMB
            deltaX[ii].append(delta)
            
    for severityToken, targetToken,ii in zip(severityCentroid, targetCentroid,range(len(targetCentroid))):
        for severityEMB, targetEMB in zip(severityToken, targetToken):
            delta = severityEMB-targetEMB
            deltaY[ii].append(delta)
            
    deltaL = np.subtract(np.array(deltaX),np.array(deltaY))
    return deltaL

def manipulate_embeddings(inputEmbeddings, SS, deltaL):
    manipulated_embeddings = inputEmbeddings.cpu().detach().numpy()
    for ii in range(len(manipulated_embeddings[0])):
        for jj in range(len(manipulated_embeddings[0][ii])):
            manipulated_embeddings[0][ii][jj] = manipulated_embeddings[0][ii][jj] + SS * deltaL[ii][jj]

    return manipulated_embeddings
\end{lstlisting}

\section{Specific Functions and Code for Improving Social Representations}
\begin{lstlisting}
def populate_embeddings(fp, clusterSize):
    embeddings = []
    with open(fp, newline='') as f:
        reader = csv.reader(f, delimiter=',')
        for row in reader:
            if len(embeddings) < clusterSize:
                embeddings.append(row)

    return embeddings
def find_cluster_centroids(embeddings):
    clusterCentroids = [[0 for i in range(len(embeddings[0])-1)] for j in range(77)]

    # get the sum
    for row in embeddings:
        for val,ii in zip(row[1:], range(len(row[1:]))):
            clusterCentroids[int(row[0])][ii]+=float(val)

    # calculate the mean
    for tokenIndex in range(len(clusterCentroids)):
        for emb, ii in zip(clusterCentroids[tokenIndex], range(len(clusterCentroids[tokenIndex]))):
            clusterCentroids[tokenIndex][ii] = emb/(len(embeddings)/len(clusterCentroids))

    return clusterCentroids
    
def calculate_deltas(embedding, cluster):
    dX= [[] for i in range(len(embedding))]
    for targetToken, inputToken,ii in zip(cluster, embedding,range(len(embedding))):
        for targetEMB, inputEMB in zip(targetToken, inputToken):
            delta = targetEMB-inputEMB
            dX[ii].append(delta)
            
    return dX
    
def transform_attribute(inputEmbs, delta, ss):
    manipulated_embeddings = inputEmbs
    for ii in range(len(manipulated_embeddings[0])):
        for jj in range(len(manipulated_embeddings[0][ii])):
            manipulated_embeddings[0][ii][jj] = manipulated_embeddings[0][ii][jj] + ss * delta[ii][jj]
    return manipulated_embeddings
    
def manipulate_gender(inputEmb, shifts, centroids):
    dM = calculate_deltas(inputEmb.tolist()[0], centroids[0])
    manipulated_embeddings = transform_attribute(inputEmbs.cpu().detach().numpy(), dM, shifts[0])
    
    dF = calculate_deltas(manipulated_embeddings.tolist()[0], centroids[1])
    manipulated_embeddings = transform_attribute(manipulated_embeddings,dF, shifts[1])
    return manipulated_embeddings

def manipulate_age(inputEmb, shifts, centroids):
    dY = calculate_deltas(inputEmb.tolist()[0], centroids[0])
    manipulated_embeddings = transform_attribute(inputEmb, dY, shifts[0])
    
    dO = calculate_deltas(manipulated_embeddings.tolist()[0], centroids[1])
    manipulated_embeddings = transform_attribute(manipulated_embeddings,dO, shifts[1])
    return manipulated_embeddings

def manipulate_race(inputEmb, shifts, centroids):
    dW = calculate_deltas(inputEmb.tolist()[0], centroids[0])
    manipulated_embeddings = transform_attribute(inputEmb, dW, shifts[0])
    
    dB = calculate_deltas(manipulated_embeddings.tolist()[0], centroids[1])
    manipulated_embeddings = transform_attribute(manipulated_embeddings,dB, shifts[1])
    
    dA = calculate_deltas(manipulated_embeddings.tolist()[0], centroids[2])
    manipulated_embeddings = transform_attribute(manipulated_embeddings,dA, shifts[2])
    return manipulated_embeddings
    
... 
...
# In main inference loop
severities = [-0.3,-0.2,-0.1,0.0,0.1,0.2,0.3] 
BALANCING_TASK = 'gender'
for ii in range(len(severities)):
    for jj in range(len(severities)):
        # for kk in range(len(severities)):   # UNCOMMENT if BALANCING_TASK == 'race'
        if BALANCING_TASK == 'gender':
            [s1,s2] = [severities[ii],severities[jj]]
        else:
            [s1,s2] = [<tuned_s1>,<tuned_s2>]    # or [0,0]
        if BALANCING_TASK == 'age':
            [s3,s4] = [severities[ii],severities[jj]]
        else:
            [s3,s4] = [<tuned_s3>,<tuned_s4>]    # or [0,0]
        if BALANCING_TASK == 'race':
            [s5,s6,s7] = [severities[ii],severities[jj],severities[kk]]   
        else:
            [s5,s6,s7] = [0,0,0] # or [<tuned_s5>,<tuned_s6>,<tuned_s7>] if doing an additional tuning loop.
        ...
        ...
        for randomSeed in randomSeeds:
            prompt = ['a picture of a person']
            batch_size = len(prompt)
        
            outputFile = outputDirectory+prompt[0]+'_'+str(randomSeed)+'-seed_'+str(s1)+'_'+str(s2)+'_'+str(s3)+'_'+str(s4)+'_'+str(s5)+'_'+str(s6)+'_'+str(s7)+'-shift.png'
            if not os.path.isfile(outputFile):
                text_input = tokenizer(prompt, padding="max_length", max_length=tokenizer.model_max_length, 
                                       truncation=True, return_tensors="pt")
                text_embeddings = text_encoder(text_input.input_ids.to(torch_device))[0]
                manipulated_embeddings = manipulate_gender(text_embeddings, [s1,s2], [maleCentroid,femaleCentroid])
                manipulated_embeddings = manipulate_age(manipulated_embeddings, [s3,s4], [youngCentroid,oldCentroid])
                manipulated_embeddings = manipulate_race(manipulated_embeddings, [s5,s6,s7], [whiteCentroid,blackCentroid,asianCentroid])
                manipulated_embeddings = torch.from_numpy(manipulated_embeddings).to(torch_device)
        ...
        # Diffusion/image generation code as in precise prompt engineering code
        ...
\end{lstlisting}
